# Supplementary material for: Quantized transconductance emerges from non-symmetric quantum fluctuations: theoretical prediction
Source: arXiv:2512.05813 ancillary file (2026-09-25)
Supplement: Supplementary file 1 [file supplementary.pdf]

# Supplemental Material for "Quantized transconductance emerges from non-symmetric quantum fluctuations: theoretical prediction"

K. Mertiri, Yuli V. Nazarov
*Kavli Institute of Nanoscience, Delft University of Technology, 2628 CJ Delft, The Netherlands*

## SUMMARY OF SUPPLEMENTAL MATERIAL

In this Supplemental Material, we provide a thorough derivation of the renormalization equation for the scattering matrix (Eq. 3 of the main text) in Section I. We also give the details of stability analysis for non-trivial fixed points (Section II), provide numerical results that illustrate the switches of transconductance (Section III), and analyze the occurrence of a jump in the probability to reach a fixed point upon crossing a stability threshold (Section IV).

## I. DERIVATION

### A. Generating Function of Full Counting Statistics

To study the renormalization of the scattering matrix, it is convenient to evaluate a physical quantity that depends on all the relevant details of the scattering matrix. In quantum transport, the proper quantity is the generating function of the Full Counting Statistics of charge transfers [1]. For two-terminal contacts, this way to derive the renormalization was implemented in [2]. Here, we generalize it to multi-terminal contacts.

Let us define the probability for $N_i$ charges to be transferred to terminals labeled by $i$ during a time interval $\mathcal{T}$, $P(\{N_i\})$ (we consider a very long interval $\mathcal{T} \to \infty$ to simplify calculations). The generating function of this probability distribution reads

$$\mathcal{Z}(\{\chi_i\}) = \sum_{N_i} e^{i\chi_i N_i} P(\{N_i\}), \tag{1}$$

where the parameters $\chi_i$ defined in each terminal are called counting fields. It is convenient in the process of calculation to define a separate terminal for each channel: we can always merge them in the end assigning the same $\chi_i$ to all channels in the same terminal.

To obtain the expression for $\mathcal{Z}(\{\chi_i\})$ in our setup, we follow [3]. We ascribe the constant voltages $V_i$, applied at the terminals, to the energy shifts of the electron filling factors with respect to their equilibrium value, $f_i(\epsilon) \to f_{\rm eq}(\epsilon - eV_i)$. The fluctuating voltages $v_i(t)$ induced by the external electromagnetic environment affect the phases of the scattering matrix making it time-dependent (we set $\hbar = 1$):

$$s_{ij} \to s_{ij}(t) = e^{-i\phi_i(t)} s_{ij} e^{i\phi_j(t)};\ \partial_t \phi_i(t) = ev_i(t). \tag{2}$$

The generating function is obtained in the Keldysh technique as a path integral over the fields $\phi_i^{\pm}(t)$ corresponding to the two parts of the Keldysh contour.

$$\mathcal{Z}(\{\chi_i\}) = \int \prod_{0<t<\mathcal{T}} d\phi_i^+(t) d\phi_i^-(t) \exp\{A_{\rm s}\left[\{\chi_i\}, \phi_i^{\pm}(t)\right] + A_{\rm env}\left[\phi_i^{\pm}(t)\right]\}. \tag{3}$$

The Keldysh action $A_{\rm s}$ of a multi-terminal scatterer is derived in [3]. We write $A_s$ in a compact form by introducing the matrices in the space of time and channels: $\chi$ is diagonal in channel space not depending on time, $f$ is diagonal in channel and energy representation, $\phi^{\pm}$ are diagonal in channel and time representation, and $s^{\pm} = e^{-i(\phi^{\pm} - \chi/2)} s e^{i(\phi^{\pm} - \chi/2)}$ is diagonal in time representation. With this,

$$A_{\rm s} = {\rm Tr}[\ln(s^-(1-f) + s^+ f)] - {\rm Tr}[\ln s^-]. \tag{4}$$

The Keldysh action $A_{\rm env}$ of the linear electromagnetic environment is quadratic in $\phi^{\pm}$ and gives rise to the following correlators of the phases, $K_{ab}^{\alpha\beta}(t) = \langle \phi_a^{\alpha}(t) \phi_b^{\beta}(0) \rangle$:

$$K_{ab}^{+-}(\omega) = -i[\chi_{ab}(\omega) - \chi_{ba}^*(\omega)]N(\omega); \quad K_{ab}^{-+}(\omega) = -i[\chi_{ab}(\omega) - \chi_{ba}^*(\omega)](1 + N(\omega); \tag{5}$$

$$K_{ab}^{++}(\omega) = -i[\chi_{ab}(\omega)(1 + N(\omega)) - \chi_{ba}^*(\omega) N(\omega)]; \quad K_{ab}^{--}(\omega) = i[-\chi_{ab}(\omega) N(\omega) + \chi_{ba}^*(\omega)(1 + N(\omega)], \tag{6}$$

where $N(\omega) \equiv \frac{1}{2}\left(\coth(\omega/2k_BT) - 1\right)$ coincides with the Bose-Einstein distribution at $\omega > 0$, and $\chi_{ab}(\omega)$ is the matrix of the dynamical susceptibilities of $\phi_a$, readily expressed in terms of the impedance matrix $\chi_{ab}(\omega) = ie^2 Z_{ab}(\omega)/\omega$.

At large $\mathcal{T}$, $\mathcal{Z}(\{\chi_i\}) = \exp(\mathcal{F}(\{\chi_i\})\mathcal{T})$, $\mathcal{F}(\{\chi_i\})$ not depending on $\mathcal{T}$. If we neglect the fluctuations,

$$\mathcal{F}_0 = \int \frac{d\epsilon}{2\pi} \det[s^-(1-f(\epsilon)) + s^+ f(\epsilon)]/\det[s^-] = \int \frac{d\epsilon}{2\pi} \det[1 + (s^\dagger e^{i\chi} s e^{-i\chi} - 1) f(\epsilon)], \tag{7}$$

in accordance with Ref. [1].

### B. First-order fluctuation correction

Let us compute the first-order fluctuation correction to $\mathcal{F}$. It is instructive to do the computation for a more general model. Namely, we consider a scattering matrix $s(\{x_a\})$ that depends on a set $x_a$ of general parameters and account for the fluctuations of the parameters. For the first-order fluctuation corrections, it suffices to expand the scattering matrix around the equilibrium value $x_a = 0$,

$$s(\{x_a\}) = s + s_a x_a + \frac{1}{2} s_{ab} x_a x_b + \ldots;\ s_a \equiv \partial_{x_a} s. \tag{8}$$

It is worth noting that the unitarity of the scattering matrix implies

$$s^\dagger s_a + s_a^\dagger s = 0;\ s^\dagger s_{ab} + s_{ab}^\dagger s + s_b^\dagger s_a + s_a^\dagger s_b = 0. \tag{9}$$

We substitute $s^\pm(t) = e^{\pm i\chi/2} s(\{x_a^\pm(t)\}) e^{\mp i\chi/2}$ into the expression for $\mathcal{Z}(\{\chi_i\})$ and expand in $x_a^\pm$.

The first-order fluctuation correction then reads:

$$\mathcal{F}^{(1)}(\{\chi_i\})\mathcal{T} = \langle A_2 \rangle + \frac{1}{2}\langle A_1^2 \rangle, \tag{10}$$

$$A_1 \equiv \mathrm{Tr}[(\delta s^+ (s^+)^\dagger - \delta s^- (s^-)^\dagger) D^+] = \mathrm{Tr}[(x_a^+ s_a^+ (s^+)^\dagger - x_a^- s_a^- (s^-)^\dagger) D^+], \tag{11}$$

$$A_2 = \frac{1}{2}\,\mathrm{Tr}\left[\left(x_a^+ x_b^+ s_{ab}^+ (s^+)^\dagger - x_a^- x_b^- s_{ab}^- (s^-)^\dagger\right) D^+\right]$$
$$-\frac{1}{2}\,\mathrm{Tr}\left[\left(x_a^- s_a^- (s^-)^\dagger D^- + x_a^+ s_a^+ (s^+)^\dagger D^+\right)\left(x_b^- s_b^- (s^-)^\dagger D^- + x_b^+ s_b^+ (s^+)^\dagger D^+\right) - x_a^- s_a^- (s^-)^\dagger x_b^- s_b^- (s^-)^\dagger\right], \tag{12}$$

where the averaging is over the fluctuations of $x_a$, $D^\pm = s^\pm f^\pm (s^- f^- + s^+ f^+)^{-1}$, $f^\pm = f, (1-f)$ is diagonal in energy representation. We note that the term $\propto \langle A_1^2 \rangle$ contains only zero-frequency correlators of $x_a$. This term describes the modification of FCS at low frequencies investigated in [4], which is a separate effect not related to the renormalization of the scattering matrix. To this end, we skip this term and write down the correction in energy representation,

$$\mathcal{F}^{(1)}(\{\chi_i\}) = \frac{1}{2}\mathcal{T}\int \frac{d\epsilon}{2\pi}\frac{d\omega}{2\pi}\left\{K_{ab}^{++}(\omega)\mathrm{Tr}\left[s_{ab}^+ (s^+)^\dagger D^+(\epsilon) - s_a^+ (s^+)^\dagger D^+(\epsilon-\omega) s_b^+ (s^+)^\dagger D^+(\epsilon)\right]\right. \tag{13}$$
$$-K_{ab}^{--}(\omega)\mathrm{Tr}\left[s_{ab}^- (s^-)^\dagger D^+(\epsilon) + s_a^- (s^-)^\dagger D^-(\epsilon-\omega) s_b^- (s^-)^\dagger D^-(\epsilon) - s_a^- (s^-)^\dagger s_b^- (s^-)^\dagger\right]$$
$$\left.+K_{ab}^{-+}(\omega)\mathrm{Tr}\left[s_a^- (s^-)^\dagger D^-(\epsilon-\omega) s_b^+ (s^+)^\dagger D^+(\epsilon)\right] + K_{ab}^{+-}(\omega)\mathrm{Tr}\left[s_a^+ (s^+)^\dagger D^+(\epsilon-\omega) s_b^- (s^-)^\dagger D^-(\epsilon)\right]\right\}.$$

This expression contains the contributions of inelastic processes as well as the renormalization of the elastic scattering amplitudes. To single out the latter, we model the filling factors as follows: Electrons fill all negative energy levels, $f(\epsilon < 0) = 1$, and all levels above some energy $E$ are empty, $f(\epsilon > E) = 0$. For $0 < \epsilon < E$, the filling factors are assumed to be arbitrary. The energy scale $E$ is in practice determined by the maximum bias voltage between the leads and/or the temperature. The field fluctuations renormalize the scattering matrix for the interval $(0, E)$. To concentrate on elastic contributions, we restrict integration over the environmental modes by $|\omega| > E$. With this, the correction reduces to

$$\mathcal{F}^{(1)}(\{\chi_i\}) = \int_0^E \frac{d\epsilon}{2\pi}\int_E^\infty \frac{d\omega}{2\pi}\left\{K_{ab}^{++}(\omega)\mathrm{Tr}\left[s_{ab}^+ (s^+)^\dagger - s_a^+ (s^+)^\dagger s_b^+ (s^+)^\dagger\right] - K_{ba}^{--}(\omega)\mathrm{Tr}\left[s_{ab}^- (s^-)^\dagger - s_a^- (s^-)^\dagger s_b^- (s^-)^\dagger\right]\right.$$
$$\left.+K_{ba}^{+-}(\omega)\mathrm{Tr}\left[s_a^- (s^-)^\dagger s_b^+ (s^+)^\dagger - s_a^- (s^-)^\dagger s_b^+ (s^+)^\dagger\right]\right\} D^+(\epsilon). \tag{14}$$

We take the limit of low temperatures $E \gg k_B T$, so that $K^{+-} = 0$, and the correction simplifies to:

$$i\mathcal{F}^{(1)}(\{\chi_i\}) = \int_0^E \frac{d\epsilon}{2\pi} \int_E^\infty \frac{d\omega}{2\pi} \left(\chi_{ab}(\omega)\mathrm{Tr}\left[\left(s^+_{ab} - s^+_a (s^+)^\dagger s^+_b\right)(s^+)^\dagger D^+(\epsilon)\right]\right.$$
$$\left. +\chi^*_{ab}(\omega)\mathrm{Tr}\left[\left(s^-_{ab} - s^-_a (s^-)^\dagger s^-_b\right)(s^-)^\dagger D^+(\epsilon)\right]\right). \tag{15}$$

We note that the integration of $\mathrm{Re}\,\chi_{ab}(\omega)$ gives zero, as the system admits no instantaneous response

$$\int_0^\infty d\omega \mathrm{Re}\chi_{ab}(\omega) = \frac{1}{2}\mathrm{Re}\int_{-\infty}^\infty d\omega \chi_{ab}(\omega) = \frac{i}{2}\langle \hat{x}_a\hat{x}_b - \hat{x}_b\hat{x}_a\rangle = 0, \tag{16}$$

so we replace $\chi_{ab}$ with its imaginary part.

Now we need to show that this correction can be presented as a change of the scattering. To this end, we compare eq. (15) and eq. (11), and prove that the change reads:

$$\delta s = \frac{1}{2\pi}\int_E^\infty d\omega\, \mathrm{Im}\,\chi_{ab}(\omega)(s_{ab} - s_a s^\dagger s_b). \tag{17}$$

This change satisfies the unitarity of $s$.

### C. Renormalization

The further interpretation of the result (17) depends on the frequency dependence of $\chi_{ab}$. If the integral over $\omega$ converges, it gives a small perturbative correction to the scattering matrix.

However, it is not the case of the setup under consideration. For a scatterer in an Ohmic environment, $\mathrm{Im}\,\chi_{ab}(\omega) = e^2 Z_{ab}/\omega = 2\pi z_{ab}/\omega$, where we define the dimensionless impedance matrix $z_{ab}$. The integral defining $\delta s$ diverges logarithmically at the lower limit. This indicates the break-down of perturbation theory at sufficiently small energies. To deal with this, we employ a renormalization procedure. At each step of the renormalization, we change $E$ by $dE$ and $s$ by $\delta s$ coming from the intergation over a small interval of $\omega$, $E > \omega > E - dE$. This results in the following differential equation for the $E$ and $\phi$-dependent scattering matrix:

$$-E\frac{\partial s(E, \{\phi_a\})}{\partial E} = \sum_b z_{ab}\left(\frac{\partial^2 s}{\partial\phi_b\partial\phi_a} - \frac{\partial s}{\partial \phi_a}s^\dagger\frac{\partial s}{\partial\phi_b}\right). \tag{18}$$

It is convenient to introduce a dimensionless variable $\xi = \ln(E_{\mathrm{cut}}/E)$ ($\xi = 0$ at the upper cut-off energy, $\xi \to \infty$ if $E \to 0$) and recall the assumption of a separate terminal for each channel, so $\phi$'s are labeled with $i$ labeling the channels.

We solve Eq. (18) with the following Ansatz specifying the phase dependence of the scattering matrix: $s_{ij}(\{\phi_a\}) = e^{-i\phi_i}s_{ij}(\xi)e^{i\phi_j}$. This gives us the following equation for $s$:

$$\frac{ds_{ij}(\xi)}{d\xi} = z_{ji}s_{ij} - \sum_{k,l} z_{kl}s_{ik}(s^\dagger)_{kl}s_{lj}. \tag{19}$$

Thereby we have completed the derivation of Eq. 3 in the main text.

## II. STABILITY ANALYSIS OF THE NON-TRIVIAL FIXED POINTS

In this Section, we analyze the stability of the fixed points of the renormalization flow equation (19) that correspond to non-trivial permutations of channels. We start from the expression of the pseudo-potential (Eq. 7 of the main text)

$$\varepsilon = -\sum_{ik} z_{ki}|s_{ik}|^2. \tag{20}$$

We substitute $\hat{s}$ in the form $\hat{s} = e^{i\hat{\theta}_1}\hat{P}\hat{U}e^{i\hat{\theta}_2}$ where irrelevant phase matrices $\hat{\theta}_{1,2}$ are diagonal in channel space, $\hat{P}$ is a permutation matrix corresponding to the fixed point under consideration, $\hat{U}$ is a unitary matrix ($\hat{U} = 1$ at the point).

We present $\hat{U} = e^{i\hat{h}}$ the Hermitian matrix $\hat{h}$ characterizing the deviation from the fixed point. We expand $\varepsilon$ to second order in $\hat{h}$ and arrive at:

$$\varepsilon = -\mathrm{Tr}[\hat{z}\hat{P}] + \sum_{kl} \left( (\hat{z}\hat{P})_{kk} - (\hat{z}\hat{P})_{kl} \right) |h_{kl}|^2. \tag{21}$$

The terms of first order in $\hat{h}$ vanish, manifesting that this is a fixed point. The stability implies that the sum of second-order terms is positively defined, that is,

$$(\hat{z}\hat{P})_{ii} + (\hat{z}\hat{P})_{jj} > (\hat{z}\hat{P})_{ij} + (\hat{z}\hat{P})_{ji} \quad \forall i, j. \tag{22}$$

This corresponds to Eq. 6 of the main text. It is worth noting that although condition (22) is one of the conditions required for $\hat{z}\hat{P}$ to be positively defined, this is not in general case and in many examples we have studied (22) numerically.

Any permutation can be decomposed into disjoint cycles. The conditions (22) should be fulfilled for $i, j$ within each cycle as well as for $i, j$ that belong to different cycles. Let us analyze cycles of various lengths $n$. For any $i, k$ that belong to (different) cycles of the length $n = 1$ the stability is guaranteed by the positivity of the impedance matrix,

$$(\hat{z}\hat{P})_{ii} + (\hat{z}\hat{P})_{jj} - (\hat{z}\hat{P})_{ij} - (\hat{z}\hat{P})_{ji} \to z_{ii} + z_{jj} - z_{ij} - z_{ji} > 0. \tag{23}$$

Let us consider a cycle with $n = 2$ corresponding to permutation $k \to l, l \to k$. For this pair of indices,

$$(\hat{z}\hat{P})_{kk} + (\hat{z}\hat{P})_{ll} - (\hat{z}\hat{P})_{kl} - (\hat{z}\hat{P})_{lk} \to z_{kl} + z_{lk} - z_{kk} - z_{ll} < 0, \tag{24}$$

that is, the positivity of $\hat{z}$ implies that any $\hat{P}$ containing a cycle $n = 2$ is automatically *unstable*.

Let us investigate the stability of a general cycle of the length $n$. It is convenient to renumber the indices within the cycle such that $P_{ki} = \delta_{k,i-1}$ (assuming a cyclic shift, so that $i - 1 = n$ if $i = 1$). We have $n(n-1)/2$ independent inequalities

$$z_{i,i-1} + z_{j,j-1} > z_{i,j-1} + z_{j,i-1} \quad \forall i \neq j, \tag{25}$$

imposed on $n$ quantities $z_{i,i-1}$ on the LHS of the inequalities. It is crucial to note that for $n > 2$ all conjugated quantities $z_{i-1,i}$ are on the RHS. Let us start with an arbitrary $z$ and increase $z_{i,i-1}$ while decreasing $z_{i-1,i}$, $z_{i,i-1} \to z_{i,i-1} + c_i$, $z_{i-1,i} \to z_{i-1,i} - c_i$, $c_i > 0$. This changes the anti-symmetric part of $\hat{z}$ only, thus not affecting its positivity. We see that the LHS of all inequalities increases while the RHS either decreases or stays the same. If the stability conditions are not fulfilled for an initial $\hat{z}$, they all become fulfilled at sufficiently big $c_i$. We can generalize this reasoning: *any permutation, not containing cycles of* $n = 2$, *gives rise to a stable fixed point at sufficiently big anti-symmetric part of* $\hat{z}$.

Let us give a more detailed analysis of several cycles of short length. For $n = 3$ (the case we have extensively exemplified with numerical calculations), there are 3 conditions:

$$z_{13} + z_{21} > z_{11} + z_{23}; \quad z_{21} + z_{32} > z_{22} + z_{31}; \quad z_{32} + z_{13} > z_{33} + z_{12}; \tag{26}$$

the second and third are obtained from the first by cyclic permutation of indices. It is convenient to separate $\hat{z}$ into a symmetric and anti-symmetric part, $\hat{z} = \hat{z}^A + \hat{z}^S$. Substituting this into (26), we observe that all three conditions are imposed on the same quantity $A \equiv z^A_{21} + z^A_{32} + z^A_{13}$,

$$A > X_1, X_2, X_3; \quad X_1 \equiv z_{11} + z^S_{23} - z^S_{13} - z^S_{21}, \tag{27}$$

$X_{2,3}$ are obtained by cyclic permutation of indices. $X_{1-3}$ can be either positive or negative. However, we note that

$$X_1 + X_2 + X_3 = z_{11} + z_{22} + z_{33} - z^S_{12} - z^S_{23} - z^S_{31} > \frac{z_{11} + z_{22} + z_{33}}{2} > 0. \tag{28}$$

Therefore, at least one of $X_{1-3}$ must be positive and $A$ is restricted by a positive quantity. This implies that *any permutation containing an* $n = 3$ *cycle is stable only if* $z$ *is non-symmetric.*

For a simple few-parameter illustration, we will use special $\hat{z}$ matrices that are invariant with respect to cyclic permutation of indices,

$$z_{i,i+m} = K_m \quad \forall i;\ |m| \leq n/2, \tag{29}$$

and separate them into symmetric and asymmetric parts as $K_{\pm m} = \bar{K}_m \mp A_m$ (assuming $m > 0$). For $n = 3$, such a matrix has three independent elements: $K_0$, $\bar{K}_1$, $A_1$, positivity impies $K_0 > 0$, $|\bar{K}_1| < K_0$, and the stability condition reads

$$3A_1 > K_0 - \bar{K}_1 > 0. \tag{30}$$

Let us turn to the case of $n = 4$. There are 6 conditions on the elements of $\hat{z}$:

$$z_{14} + z_{21} > z_{11} + z_{24} \text{ and 3 cyclic permutations;} \tag{31}$$

$$z_{14} + z_{32} > z_{12} + z_{34} \text{ and 1 cyclic permutation.} \tag{32}$$

Let us see if these conditions can be satisfied with a *symmetric* $\hat{z}$. For this case, the two last conditions

$$z^S_{14} + z^S_{32} > z^S_{12} + z^S_{34}; \quad z^S_{21} + z^S_{43} > z^S_{23} + z^S_{41}, \tag{33}$$

can be only *marginally* satisfied provided $z^S_{14} + z^S_{32} = z^S_{12} + z^S_{34}$. So, similar to the $n = 3$ case, *any permutation containing an $n = 4$ cycle can only be stable if $\hat{z}$ is non-symmetric.*

Let us illustrate the case with the cyclic-invariant $\hat{z}$ matrices. The independent elements are $K_0, \bar{K}_1, A_1, \bar{K}_2$ (since $K_2 = K_{-2}$), positivity implies $K_0 > 0$, $|\bar{K}_{1,2}| < K_0$. The stability is satisfied by two conditions imposed on $A_1$:

$$2A_1 > K_0 + \bar{K}_2 - 2\bar{K}_1; \quad A_1 > 0. \tag{34}$$

Finally, let us consider $n = 5$. There are 10 conditions imposed on $z$:

$$z_{15} + z_{21} > z_{11} + z_{25} \text{ and 4 cyclic permutations;} \tag{35}$$

$$z_{15} + z_{32} > z_{12} + z_{35} \text{ and 4 cyclic permutation.} \tag{36}$$

Somewhat similar to $n = 3$, these conditions give rise to 5 inequalities imposed on a single quantity $A \equiv \sum_{i=1}^{5} z^A_{i,i-1}$,

$$A > X_1, X_2, X_3, X_4, X_5; \quad X_1 = z_{11} + 2z^S_{52} - z^S_{15} - z^S_{21} - z^S_{32} - z^S_{43}. \tag{37}$$

$X_{2-5}$ are obtained by cyclic permutations of indices. $X_{1-5}$ can be either positive or negative. In distinction from the $n = 3$ case, the sum of all $X$ does not have to be positive, and all 5 thresholds for $A$ can appear negative. In this situation, the conditions can be satisfied with $A = 0$. Therefore, *some symmetric $\hat{z}$ matrices may give rise to stable fixed points with cycles of $n > 5$.*

Again, we illustrate this with the cyclic-invariant $\hat{z}$ matrices. The independent elements are $K_0, \bar{K}_1, \bar{K}_2$, $A_1$, $A_2$, positivity implies $K_0 > 0$, $|\bar{K}_{1,2}| < K_0$. The stability is satisfied by two conditions imposed on $A_{1,2}$:

$$2A_1 - A_2 > K_0 + \bar{K}_2 - 2\bar{K}_1; \quad 3A_1 + A_2 > \bar{K}_2 - \bar{K}_1. \tag{38}$$

A symmetric $\hat{z}$ matrix with the non-trivial stable point satisfies

$$\bar{K}_1 > \frac{K_0 + \bar{K}_2}{2} > 0. \tag{39}$$

Thus 5-cycle stable fixed points can be realized in a wide range of engineered $\hat{z}$ matrices.

This does not mean that such matrices frequently occur if a positively defined $\hat{z}$ is chosen *at random*. Indeed, an $n$-cycle requires $n(n-1)/2$ conditions to be fulfilled. Even if each condition is fulfilled with 1/2 probability, the probability to reach stability would be $2^{-n(n-1)/2}$, that is, $10^{-3}$ for $n = 5$. To qualify this better, we perform the following simulation. We draw a random $n \times n$ matrix $\hat{a}$ with elements uniformly distributed in the interval $(-1, 1)$. We form a positively defined symmetric $\hat{z} = \hat{a}^T\hat{a}$, check the conditions (22) for a given $n$-cycle permutation, and accumulate the statistics of successful draws. For $n = 5$ and a given permutation, we find the probability of success $p_s = 6.7 \times 10^{-6}$. One has to take into account that there are $(n-1)! = 24$ possible permutations of this form, therefore the total probability of success for any possible fixed point is $p_t(5) = 1.6 \times 10^{-4}$. We perform the same simulations for $n = 6$ and $n = 7$ to find yet smaller total probabilities $p_t(6) = 6.2 \times 10^{-5}$, $p_t(7) = 1.4 \times 10^{-6}$.

## III. ILLUSTRATIONS OF RENORMALIZATION FLOW: SWITCHES

It is an important result of our paper that the fixed point describing the low-energy transport crucially depends on both the initial configuration of the scattering matrix and the parameters defining the asymmetry of the impedance

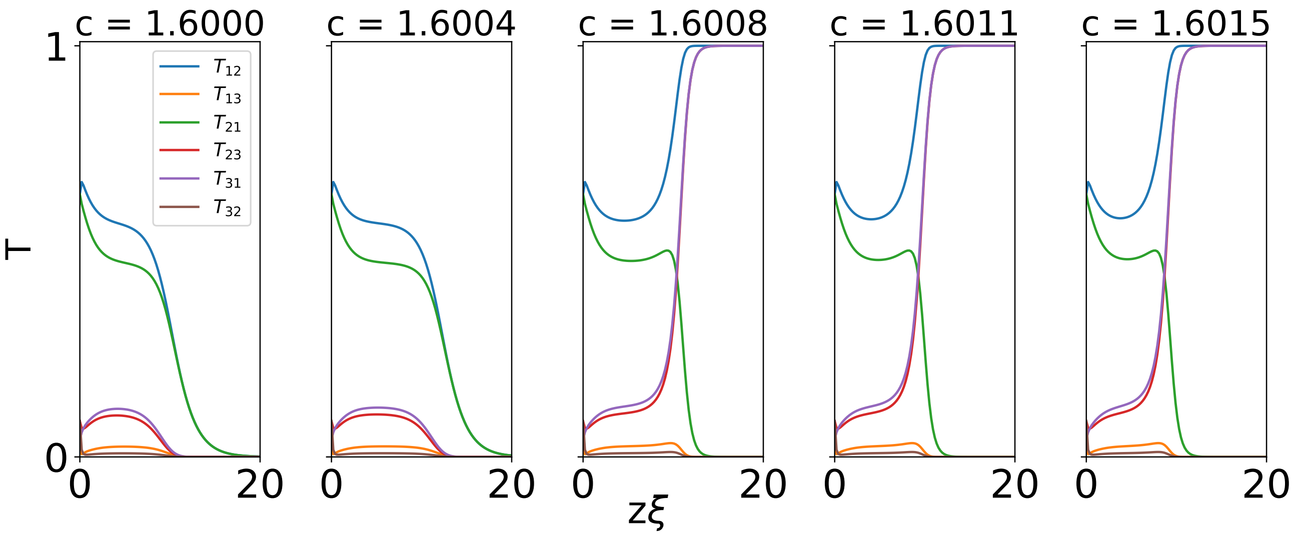


FIG. 1. The transconductance switch upon changing the environment. The 3-terminal setup, 1 channel per terminal. The renormalization flow for the impedance matrix specified in the text at the parameter $c$ varying in a narrow interval. The initial scattering matrix is the same for all the plots.

matrix. Both can be varied experimentally within a given setup: the initial scattering matrix may be tuned by gate voltages that change the scattering potential, the impedance matrix can be changed by tuning the electromagnetic environment. A small variation can result in a sudden switch in the observed low-energy transconductances.

Firstly, we illustrate a switch upon changing the parameter $c$ in the manifold of matrices $\hat{z}$ defined in the main text. We compute the renormalization flow solving Eq. 3 of the main text at varying $c$ starting with the same $\hat{s}_{\rm in}$. The results are presented in Fig. 1. We choose a narrow interval of $c$ where the switch takes place. We plot the trasconductances in the interval $z\xi = [0, 20]$. For the two leftmost plots, the limiting values of transcondutances are 0 corresponding to insulation. The switch happens between $c = 1.6004$ and $c = 1.6008$. For the three rightmost plots, the limiting values $T_{12} = T_{23} = T_{31} = 1$ manifest a QTC fixed point. We see that the energy dependence of the transmission coefficients hardly changes from plot to plot in the interval $z\xi = [0, 10]$, while switching between the fixed points in the interval $z\xi = [10, 20]$.

We note that the $c$ value corresponding to a switch differs for different $\hat{s}_{\rm in}$ and does not generally coincide with the threshold $c_s$ seen in the statistics of the fixed points.

Another illustration we make involves the 3-terminal setup with 10 channels per terminal. We plot in Fig. 2 the transconductance versus $c$ for a chosen $\hat{s}_{\rm in}$. We observe a monotonic increase of trasconductance with $c$ that proceeds with the switches. We can see that near the configuration-specific stability threshold the transconductance corresponding to a given configuration $\hat{s}_{\rm in}$ changes rapidly with $c$, while saturating at high $c$.

A switch in the low-energy transconductances can also occur upon a change in the initial scattering matrix. To illustrate, we compute and plot the transmission coefficient $T_{12}$ flow in Fig. 3 for different initial scattering matrices parametrized by $\alpha$: $\hat{s}_{\rm in}(\alpha) = e^{i\alpha\hat{\lambda}}\hat{s}_{\rm in}(0)$, $\hat{\lambda}$ being a $3 \times 3$ matrix with non-zero elements $\lambda_{12} = \lambda_{21} = 1$, and $\hat{s}_{\rm in}(0)$ being the initial scattering matrix we use to produce Fig. 1. We choose $c = 1.6$ at which this matrix evolves to the insulating fixed point. Upon changing $\alpha$ we observe a switch to ideal transconductance at $\alpha \approx 2$ in a narrow interval of $\alpha$. There is a pronounced difference between the traces at $\alpha = 2.05$ and $\alpha = 2.08$.

In Fig. 2 of the main text, we illustrate the flow for different scattering matrices $\hat{s}_{A,B}$ evolving to the insulating/QTC fixed point, respectively. Here, we investigate the line of scattering matrices that connects $A$ and $B$, $\hat{s}_{\rm in}(\alpha) = \hat{s}_A^{\alpha}\hat{s}_B^{1-\alpha}$, $\alpha = [0, 1]$. In Fig. 4, we illustrate the switch that occurs at $\alpha \approx 2.7 \times 10^{-4}$. The small value of $\alpha$ indicates that $\hat{s}_A$ is close to the stability threshold. We note the similarity with the series of plots presented in Fig. 1: the traces either above or below the threshold differ from each other only in a narrow interval $z\xi$.

## IV. PROBABILITY TO EVOLVE TO A QTC NEAR A STABILITY THRESHOLD

In the main text, we numerically evaluated the probabilities to evolve to a given QTC fixed points for $\hat{s}_{\rm in}$ drawn from the circular ensemble (see e.g. Fig 3 of the main text). Intuitively, one would expect the probability to be a

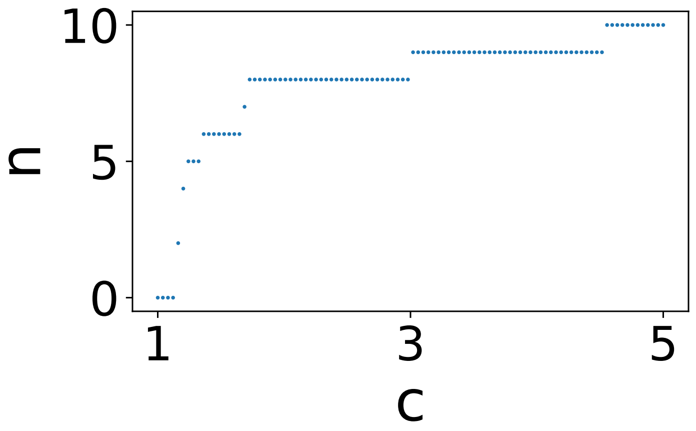


FIG. 2. The transconductance switch upon changing the environment. The 3-terminal setup, 10 channels per terminal. The initial scattering matrix is fixed for all $c$. The transconductances $G_{12} = G_{23} = G_{31}$ switch between integer multiples $n$ of $G_Q$ upon changing $c$.

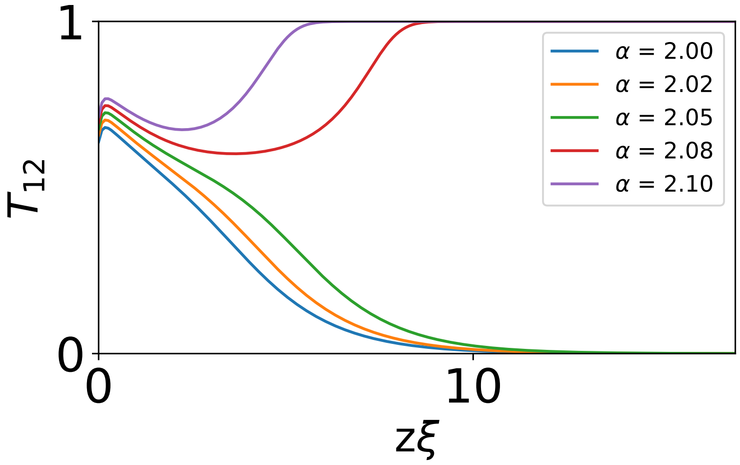


FIG. 3. The transconductance switch upon changing the initial scattering matrix. The 3-terminal setup, 1 channel per terminal. The renormalization flow of the transmission coefficient $T_{12}$ for the initial scattering matrix $\hat{s}_{\rm in}(\alpha)$ defined in the text. For this plot, $c = 1.6$.

continuous function of the parameter $c$ at the stability threshold, and thus a small probability for $c$ slightly above the threshold. In fact, Fig. 3 might suggest this. But this is not the case. More detailed simulation of the same setup in a narrow interval of $c$ near the threshold (Fig. 5) shows a jump of the probability from 0 to $\approx 0.25$ precisely at $c_s$. This is for the one channel per terminal case, yet we believe that the jumps do occur for any setup. The only point is that for a bigger number of channels ( see e.g. Fig 4b of the main text), the jumps are either small or close to 1.

To explain the result qualitatively, we investigate the form of the pseudo-potential near a stability threshold. A common prescription would suggest to concentrate on the vicinity of the fixed point and employ a polynomial expansion of the potential. This does not work for the potential in hand. To see this, let us look back at the expansion (21) and the corresponding stability conditions (22). At a threshold, one of the conditions corresponding to a pair of indices $i, j$ becomes marginal: we can always renumber the indices such that $i, j = 1, 2$ so that at the threshold

$$(\hat{z}\hat{P})_{11} + (\hat{z}\hat{P})_{22} - (\hat{z}\hat{P})_{12} - (\hat{z}\hat{P})_{21} \equiv z_c = 0, \tag{40}$$

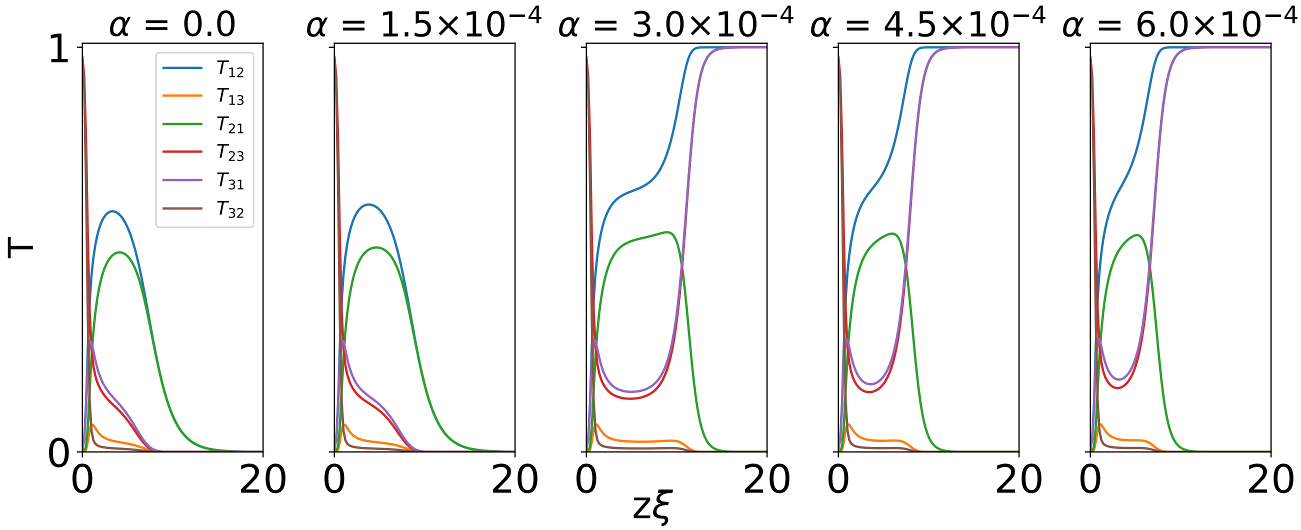


FIG. 4. The transconductance switch upon changing the initial scattering matrix. The 3-terminal setup, 1 channel per terminal. The renormalization flow for a line of initial scattering matrices parametrized by $\alpha$: $\hat{s}_A^{\alpha}\hat{s}_B^{1-\alpha}$, where $\hat{s}_{A,B}$ are the same as in Fig. 2 of the main text flowing to the insulating/QTC fixed point respectively in the low energy regime. The asymmetry parameter $c = 1.5$ for all plots.

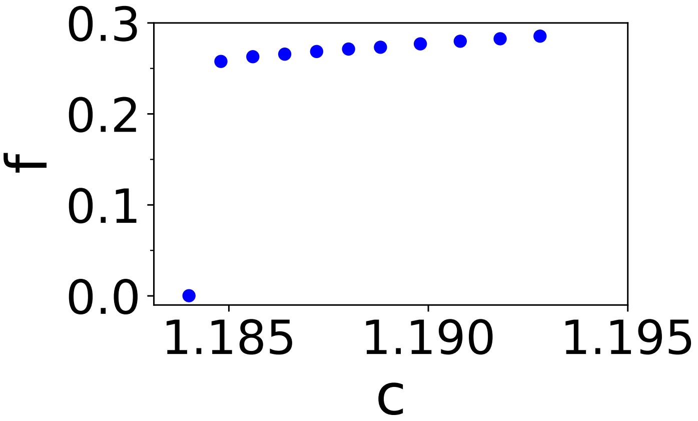


FIG. 5. One channel per terminal. The fraction of $\hat{s}_{\rm in}$ flowing to $P_1$ QTC fixed point versus asymmetry parameter $c$ near the stability threshold $c_s$ (as computed from $10^4$ runs per point in $c$ ). The fraction thus exhibits a jump at $c = c_s$.

while all other conditions are fulfilled.

The peculiarity of the pseudo-potential is that at $z_c = 0$ it takes the same value at a whole *surface* of scattering matrices $\hat{P}\hat{U}$ parameterized by a unitary $2 \times 2$ matrix $Q_{ab}$, $a, b = 1, 2$, such that $U_{ab} = Q_{ab}$, and $U_{ik} = \delta_{ik}$ for $i, k > 2$. At finite critical parameter $z_c$, the degeneracy with respect to $Q_{ab}$ is lifted. The $Q$-dependent part of the pseudo-potential reads

$$\epsilon = \mathrm{const} - z_c |Q_{12}|^2, \tag{41}$$

where we have used the unitarity of $Q_{ab}$. Above the threshold, the stable minimum corresponds to the fixed point $\hat{P}$ ($|Q_{12}|^2 = 0$). Below the threshold, the fixed point $\hat{P}$ is unstable. The minimum at the surface corresponds to an alternative fixed point $\hat{P}'$, $\hat{P}'$ obtained from $\hat{P}$ by a permutation of 1 and 2. $|Q_{12}|^2 = 1$ at this point.

In the next step, we investigate the stability of points at the surface with respect to orthogonal deviations $\hat{h}$. The

stability with respect to all $h_{ij}$ with $i, j > 2$ is already implied. We need to check the expansion in the non-diagonal elements $h_{ai}$, $i > 2$. It reads

$$\delta\varepsilon = \sum_{i,a,b} M^{(i)}_{ab} h_{bi} h^*_{ai}; \quad M^{(i)}_{ab} \equiv \sum_{c=1,2} \left( \frac{(\hat{z}\hat{P})_{bc} + (\hat{z}\hat{P})_{ac}}{2} - (\hat{z}\hat{P})_{ic} \right) Q_{ca} Q^*_{cb} + \delta_{ab} \left( (\hat{z}\hat{P})_{ii} - (\hat{z}\hat{P})_{ai} \right). \tag{42}$$

The stability is thus guaranteed if the $2 \times 2$ Hermitian matrix $M^{(i)}_{ab}$ is positively defined for all $i > 2$. It is crucial to note that the stability depends on the point of the surface. A part of the surface adjacent to $\hat{P}$ remains stable with respect to orthogonal deviations $h_{ai}$ by virtue of continuity, while a part of the surface may be unstable.

This unstable part surely exists if the point $\hat{P}'$ is unstable. If this is the case, below the threshold all renormalization trajectories go to a point with a pseudo-potential lower than that of $\hat{P}'$. Some do this directly without hitting the surface, some stick to the stable part of the surface first and slowly ($\propto |z_c|$) move towards $\hat{P}'$ leaving the surface when they achieve the unstable part. Sightly above the threshold, the trajectories hitting the surface move towards $\hat{P}$ and stick there. Therefore, a finite fraction of the trajectories reaches $\hat{P}$ above the threshold: this fraction is proportional to the area of the stable part of the surface and does not depend on the critical parameter $z_c$.

For the case in hand, $\hat{P} : 123 \to 312$. The alternative fixed point is then $\hat{P}' : 123 \to 132$ and is unstable since it contains an $n = 2$ cycle.

If there are more channels per terminal, the stability threshold involves all channels corresponding to terminals 1 and 2. In this case the degenerate surface at $z_c = 0$ is of higher dimension.

---


[1] L. S. Levitov, H. Lee, and G. B. Lesovik, Electron counting statistics and coherent states of electric current, Journal of Mathematical Physics **37**, 4845 (1996).

[2] M. Kindermann and Y. V. Nazarov, Interaction effects on counting statistics and the transmission distribution, Phys. Rev. Lett. **91**, 136802 (2003).

[3] I. Snyman and Y. V. Nazarov, Keldysh action of a multiterminal time-dependent scatterer, Phys. Rev. B **77**, 165118 (2008).

[4] M. Kindermann, Y. V. Nazarov, and C. W. J. Beenakker, Distribution of voltage fluctuations in a current-biased conductor, Phys. Rev. Lett. **90**, 246805 (2003).
